# Supplementary material for: High-Dimensional Markov-Switching Ordinary Differential Processes
Source: arXiv:2501.00087 source file (2026-11-07)
Supplement: Supplementary file 1 [file B_smooth_deprecate__.tex]

\section{Analysis for Smoothing Regression}
\subsection{Probability of Switching}
We want to calculate that the probability that a switching occurs in the neighborhood of a sampling time, $[t_n-\delta, t_n+\delta]$. It is known that the continuous time Markov chain can be viewed as a Poisson process, where the switching is viewed as a ``jump''. Consider that the coefficient of the Poisson distribution to be $\lambda = -q_{ii}$ for $i=1,\ldots, p$. Furthermore, in the homeogenous setting, the Poisson process is stationary and the probability of switching occur in two disjoint intervals are interval. 
Hence, we can write
\[
P(\text{f has no switching occur in }[t_n-\delta, t_n+\delta]) = \exp(-2\lambda \delta)=1-2\lambda\delta + o(\delta). 
\]
Therefore, we know that $P(\text{$f$ has at least one switching occur in }[t_n-\delta, t_n+\delta])\approx 2\lambda\delta $
\begin{remark}
    This suggests that if $\delta$ is a "constant" than, the probability will never converges to zero. 
\end{remark}
We define two events: 
\begin{align*}
    f_1&=\{\text{$f$ has no switching occurs in $[t_n-\delta, t_n+\delta]$}\};\\
    f_2&=\{\text{$f$ has at least one switching occurs in $[t_n-\delta, t_n+\delta]$}\}.
\end{align*}
Therefore, we can write
\begin{align*}
\EE[(\hat{f}(t_n)-f(t_n))^2]&=\EE[\EE[(\hat{f}(t_n)-f(t_n))^2\mid f]]\\
&=\EE[(\hat{f}(t_n)-f(t_n))^2\mid f_1]P(f_1)\\
&\quad + 
\EE[(\hat{f}(t_n)-f(t_n))^2\mid f_2]P(f_2)\\
&=C(1-2\lambda\delta)(\log N/N)^{2\alpha/(1+2\alpha)}(1+o(1))\\
&\quad + 2\lambda\delta *C_1
\end{align*}
\textbf{Discussion}: we have two possible solutions for calculating $C_1$. The first is to say $C_1$ is some bounded constant. This induced bias asymptotically. Another way is to assume that the whole path is Lipschitz continuous instead of $\alpha$-Holder continuous. However, this would reduce the convergence rate to $O((\log N/N)^{2/3})$. Furthermore, the function class becomes much smaller. 

 %\begin{lemma}
 %    Given $t_n$, if there is a switching occur in $[t_n-\delta, t_n+\delta]$ for some $\delta>0$. Then, 
 %    \[
 %    \EE(\hat{f}(t_n)-f(t_n))^2\leq C(\log N/N)^{2\alpha'/(1+2\alpha')}(1+o(1)),
 %    \]
 %    where $\alpha' $
 %\end{lemma}
%\begin{proof}
    
%\end{proof}
\subsection{Consistency in $\ell_\infty$ norm}
\begin{lemma}
Consider a point $t_n$ and a constant $j_1$ such that $j_1\leq j_0\leq \log N$. Consider a wavelet function $\phi$ and a $r$-regular wavelet function $\omega$ with support $\text{supp}(\phi)=\text{supp}(\omega)=[0, L]$. Let $f\in\Lambda^\alpha(M,B,m)$ with $r\geq\alpha$ and $\hat{f}$ be the thresholded wavelet estimator. Suppose that no switching occurs between $[t_n-L/2^{j_1}, t_n+L/2^{j_1}]$, then 
\[
\sup_{f\in\Lambda^\alpha(M,B,m)}\EE\rbr{\hat{f}(t_n)-f(t_n)}^2\leq C(\log N/N)^{2\alpha/(1+2\alpha)}(1+o(1)). 
\]
\end{lemma}
\begin{proof}
    Our proof stems from Theorem~4 in~\citet{brown1998wavelet} that discusses the pointwise convergence under no switching. We extend it to incorporate the case where there is a finite number of switching points outside a neighborhood of the observed point. As~\citet{brown1998wavelet} pointed out that the extension to finite switching is straightforward from Theorem~4, we complete the claim by explicitly assessing the valid region of the neighborhood. We hence make no claims of the originality of the proof. 

    Recall that $\hat{f}(t)=N^{-1/2}\sum_{i=1}^N Y_i\phi_{Ji}(t)$, where $N=2^J$. Then, we can decompose $$    \hat{f}=f(t)+\Delta(t)+r(t),$$ where
    \[
\Delta(t)=N^{-1/2}\sum_{i=1}^N f(t_i)\phi_{Ji}(t)-f(t),\quad r(t)=N^{-1/2}\sum_{i=1}^N \varepsilon_i\phi_{Ji}(t). 
    \]
    For $k=1,\ldots, 2^j,j=j_0\ldots, J$, let
    \begin{align*}
    \hat{\rho}_{jk}&=\text{sgn}\rbr{\dotp{\hat{f}}{\omega_{jk}}}\rbr{|\dotp{\hat{f}}{\omega_{jk}}|-\lambda_{jk}}_+=\text{sgn}\rbr{\rho_{jk}+d_{jk}+r_{jk}}\rbr{|\rho_{jk}+d_{jk}+r_{jk}|-\lambda_{jk}}_+,
    \end{align*}
    where $\rho_{jk}=\dotp{f}{\omega_{jk}}$, $d_{jk}=\dotp{\Delta}{\omega_{jk}}$ and $r_{jk}=\dotp{r}{\omega_{jk}}$. 
    \begin{align*}
    \hat{\xi}_{j_0k }&=\dotp{\hat{f}}{\phi_{j_0k}}=\xi_{j_0k}+d'_{j_0k}+r_{j_0k}',\quad k=1,\ldots, 2^{j_0},
    \end{align*}
    where $\xi_{j_0k}=\dotp{f}{\phi{j_0k}}$, $d'_{j_0k}=\dotp{\Delta}{\phi_{j_0k}}$ and $r'_{j_0k}=\dotp{r}{\phi_{j_0k}}$. It follows from Theorem~1 in~\citet{brown1998wavelet} that
    \begin{align}\label{eq:upper_d}
        \sum_{k=1}^{2^{j_0}}(d_{j_0k}')^2+\sum_{j=j_0}^{J-1}\sum_{k=1}^{2^j}d_{jk}^2=o(N^{-2\alpha/(1+2\alpha)})
    \end{align}

    Then, we can write
    \begin{align*}
        \EE\rbr{\hat{f}(t_n)-f(t_n)}^2&=\EE\cbr{\sum_{k=1}^{j_0}(\hat{\xi}_{j_0k}-{\xi}_{j_0k})\phi_{j_0k}(t_n)+\sum_{j=j_0}^{J-1}\sum_{k=1}^{2^j}(\hat\rho_{jk}-\rho_{jk})\omega_{jk}(t_n)+\sum_{j=J}^{\infty}\sum_{k=1}^{2^j}{\rho_{jk}\omega_{jk}(t_n)}}^2\\
        &\leq 
        \Bigg[\sum_{k=1}^{j_0}
        \cbr{\EE(\hat{\xi}_{j_0k}-{\xi}_{j_0k})^2\phi_{j_0k}^2(t_n)}^{1/2}+\sum_{j=j_0}^{J-1}\sum_{k=1}^{2^j}\cbr{\EE(\hat{\rho}_{jk}-\rho_{jk})^2\omega_{jk}^2(t_n)}^{1/2}\\
        &\quad+\sum_{j=J}^{\infty}\sum_{k=1}^{2^j}\abr{\rho_{jk}\omega_{jk}(t_n)}\Bigg]^2\\
        &=(T_1+T_2+T_3)^{2}
    \end{align*}
    For term $T_1$, we can write it as
    \begin{align*}
        T_1 &= \sum_{k=1}^{2^{j_0}}\cbr{\EE(\hat{\xi}_{j_0k}-\xi_{j_0k})^2}^{1/2}|\phi_{j_0k}(t_n)|\\
        &\leq 2^{j_0/2}\norm{\phi}_{\infty}\sum_{k=1}^{2^{j_0}}\cbr{\EE(\hat{\xi}_{j_0k}-\xi_{j_0k})^2}^{1/2}\\
        &\leq 2^{j_0/2}\norm{\phi}_{\infty}\sum_{k=1}^{2^{j_0}}\cbr{\EE(d'_{j_0k}+r'_{j_0k})^2}^{1/2}\\
        &\leq 2^{j_0/2}\norm{\phi}_{\infty}L\cbr{N^{-1}\sigma^2+\max_{k}\rbr{d_{j_0k}'}^2}^{1/2}.
    \end{align*} 
    where $L$ is the support size of $\phi$, $\text{supp}(\phi)=[0,L]$. At the $j_0$-th resolution, there will be $L$ basis functions whose supports cover the point $t_n$.

    Then, we apply~\eqref{eq:upper_d} to the right hand side of the above equation, we can conclude that
    \[
    T_1=o(N^{-\alpha/(2\alpha+1)}).
    \]
    To show $T_2$, we introduce the  set $G_j$ as
    \[
    G_j=\{k:\text{supp}(\omega_{jk}) \text{ contains at least one switching point of $f$}\}.
    \]
     Then, $T_2$ can be written as
    \begin{align*}
    T_2
    &=\sum_{j=j_0}^{J-1}\sum_{k\in G_j}\cbr{\EE(\hat{\rho}_{jk}-\rho_{jk})^2\omega_{jk}^2(t_n)}^{1/2}
    +\sum_{j=j_0}^{J-1}\sum_{k\not\in G_j}\cbr{\EE(\hat{\rho}_{jk}-\rho_{jk})^2\omega_{jk}^2(t_n)}^{1/2}\\
    &=T_{21}+T_{22}. 
    \end{align*}

    Before finding the upper bound of $T_{2}$, we claim that
    \begin{equation}\label{eq:rho_ub}
    \EE(\hat{\rho}_{jk}-\rho_{jk})^2\leq \min\cbr{(2\log N+1)\sigma^2N^{-1},{8\rho_{jk}^2+\sigma^2N^{-2}}}+10d_{jk}^2.
    \end{equation}
    To show the claim, we can write
    \[
    \EE(\hat{\rho}_{jk}-\rho_{jk})^2\leq 
    2\EE(\hat{\rho}_{jk}-\rho_{jk}-d_{jk})^2+2d_{jk}^2.
    \]
    By Lemma~3 in~\citet{brown1998wavelet}, we can write
    \[
    \EE(\hat{\rho}_{jk}-\rho_{jk}-d_{jk})^2\leq \min\cbr{(2\log N+1)\sigma^2N^{-1}, {4(\rho_{jk}^2+d_{jk}^2)+\sigma^2N^{-2}}}.
    \]
    Therefore, we can conclude~\eqref{eq:rho_ub}.  

    Apply lemma~1 in~\citet{brown1998wavelet}, we have $\rho_{jk}^2\leq C^2 2^{-j(1+2\alpha)}$ for $k\not\in G_j$. Choose $J_1=\lfloor 1/(1+2\alpha)\log_2(N/\log N)\rfloor$, then~\eqref{eq:rho_ub} can be further expressed as
    \begin{align*}
        \EE(\hat{\rho}_{jk}-\rho_{jk})^2&\leq 5\sigma^2N^{-1}\log N+10d_{jk}^2,\quad j_0\leq j\leq J_1-1,\;k\not\in G_j;\\
        \EE(\hat{\rho}_{jk}-\rho_{jk})^2&\leq 8C^2 2^{-j(1+2\alpha)}+\sigma^2N^{-2}+10d_{jk}^2,\quad J_1\leq j\leq J-1,\;k\not\in G_j.
    \end{align*}
    Then it follows that
    \begin{align*}
    T_{22} &\leq  \sum_{j=j_0}^{J_1-1}L 2^{j/2}\|\omega\|_{\infty}(5\sigma^2N^{-1}\log N+10d_{jk}^2)^{1/2}\\
    &\quad+\sum_{j=J_1}^{J-1}L 2^{j/2}\|\omega\|_{\infty}(8C^2 2^{-j(1+2\alpha)}+\sigma^2N^{-2}+10d_{jk}^2)^{1/2}
    \end{align*}
    We have
    \[
    \abr{d_{jk}}=\abr{\dotp{\Delta}{\omega_{jk}}}\leq\norm{\omega_{jk}}_1\sup_{t\in\text{supp}(\omega_{jk})}|\Delta(t)|\leq 2^{-j/2}\norm{\omega}_1 C_0 n^{-\min(\alpha,1)}=C_1 2^{-j/2}n^{-\min(\alpha,1)},
    \]
    for $k\not\in G_j$ and $j=j_0,\ldots, J-1$. 
    Then, we can use the above result to show that
    \[
    T_{22}=O((\log N/N)^{\alpha/(2\alpha+1)}).
    \]
    
    By construction, no switching occurs between $[t_n-L/2^{j_1},t_n+L/2^{j_1}]$ for some constant $j_1$  that $j_0\leq j_1\leq J$. Hence, we can write
    \begin{align*}
    T_{21} &= \sum_{j=j_0}^{j_1-1}\sum_{k\in G_j}\cbr{\EE(\hat{\rho}_{jk}-\rho_{jk})^2\omega_{jk}^2(t_n)}^{1/2} + \sum_{j=j_1}^{J}\sum_{k\in G_j}\cbr{\EE(\hat{\rho}_{jk}-\rho_{jk})^2\omega_{jk}^2(t_n)}^{1/2}\\
    &=\sum_{j=j_0}^{j_1-1}\sum_{k\in G_j}\cbr{\EE(\hat{\rho}_{jk}-\rho_{jk})^2\omega_{jk}^2(t_n)}^{1/2}\\
    &\leq 2^{j_1/2}\norm{\omega}_\infty \sum_{j=j_0}^{j_1-1}\cbr{(2\log N+1)\sigma^2 N^{-1}+10d_{jk}^2}^{1/2}=o(N^{-\alpha/(1+2\alpha)}),
    \end{align*}
    followed by~\eqref{eq:upper_d}. 
    Next, we want to find a valid upper bound for $T_3$. Since, $2^J\geq 2^{j_1}$, there is no switching point on the interval $[t_n-L/2^j,t_n+L/2^j]$ for $j\geq J$. Therefore, we can apply Lemma~1 in~\citet{brown1998wavelet} to $T_3$ and show that
    \[
    T_3 = \sum_{j=J}^\infty\sum_{k=1}^{2^j}\abr{\rho_{jk}}\abr{\omega_{jk}(t_n)}\leq \sum_{j=J}^\infty L 2^{j/2}\norm{\omega}_{\infty}C2^{-j(1+\alpha)}\leq C' n^{-\alpha}. 
    \]
    Then, combining the results of $T_1$, $T_2$, $T_3$, we can conclude that
    \[
    \EE\rbr{\hat{f}(t_n)-f(t_n)}^2\leq C(\log N/N)^{2\alpha/(1+2\alpha)}(1+o(1)). 
    \]
\end{proof}

\subsection{Auxiliary Lemmas}
